# Supplementary material for: Rendering Anywhere You See: Renderability Field-guided Gaussian Splatting
Source: arXiv:2504.19261 source file (2025-04-27)
Supplement: Supplementary file 1 [file appendix.tex]

\clearpage
\setcounter{page}{1}
\maketitlesupplementary

This appendix provides supplementary details to support the main text, including physical interpretations of the renderability metrics, a detailed experimental setup, explanations of missing data, and ablation studies. These details aim to ensure reproducibility and offer deeper insights into the performance of our proposed methodology.

\section{Explaination of The Renderability Metrics}

The renderability field aims to filter out perspectives with poor synthesis quality. Based on this, the three introduced metrics address different cases of composition degradation. The first metric is defined as follows:
\begin{equation}\label{eee}\left.H^p_{geo}=\left\{\begin{array}{ll}1-\frac{\sum_{v_i,v_j\in \boldsymbol{I_s},i\neq j}||c(v_i,p)-c(v_j,p)||_2}{\sqrt{3} \cdot \frac{N \cdot (N-1)}{2}},&N > 1,\\1,&N \leq 1.\end{array}\right.\right.\end{equation}

This metric addresses non-Lambertian surfaces, such as highly reflective objects, where the mean color disparity across multiple views is significant, leading to the degradation of Gaussian primitives. Since the L2 norm of normalized pixel values ranges within \([0, \sqrt{3}]\), we further normalize it to ensure the metric lies between 0 and 1.

The other two metrics address view dependence and close-range blurring. When the observation directions are incomplete, Gaussian primitives, primarily fitted to the source view, tend to produce holes or spikes in other viewpoints. Additionally, image resolution about the same region decreases at greater distances, leading to insufficient optimization of geometric features and causing artifacts to appear in close-up views.

Since viewpoint positions also influence these two metrics, they are related to the first metric, encouraging a denser viewpoint distribution for non-Lambertian regions.

Guided by the three metrics mentioned above, we sampled precise pseudo-views to enhance weakly observed areas. As shown in Figure \ref{PSNR_DIS}, using PSNR$=$25 as a reference line, our method significantly reduces the number of low-quality views, and raises the lower bound of novel view synthesis quality, while maintaining the high-quality view distribution of 3D-GS. The new perspectives rendered by Octree-GS are sparse in the PSNR$>$35 range, indicating a reduction in the upper bound of rendering quality. Other methods show a clear gap compared to ours.

\begin{figure}[htp]
        \centering
	\begin{minipage}[c]{0.47\textwidth}
		\includegraphics[width=\textwidth]{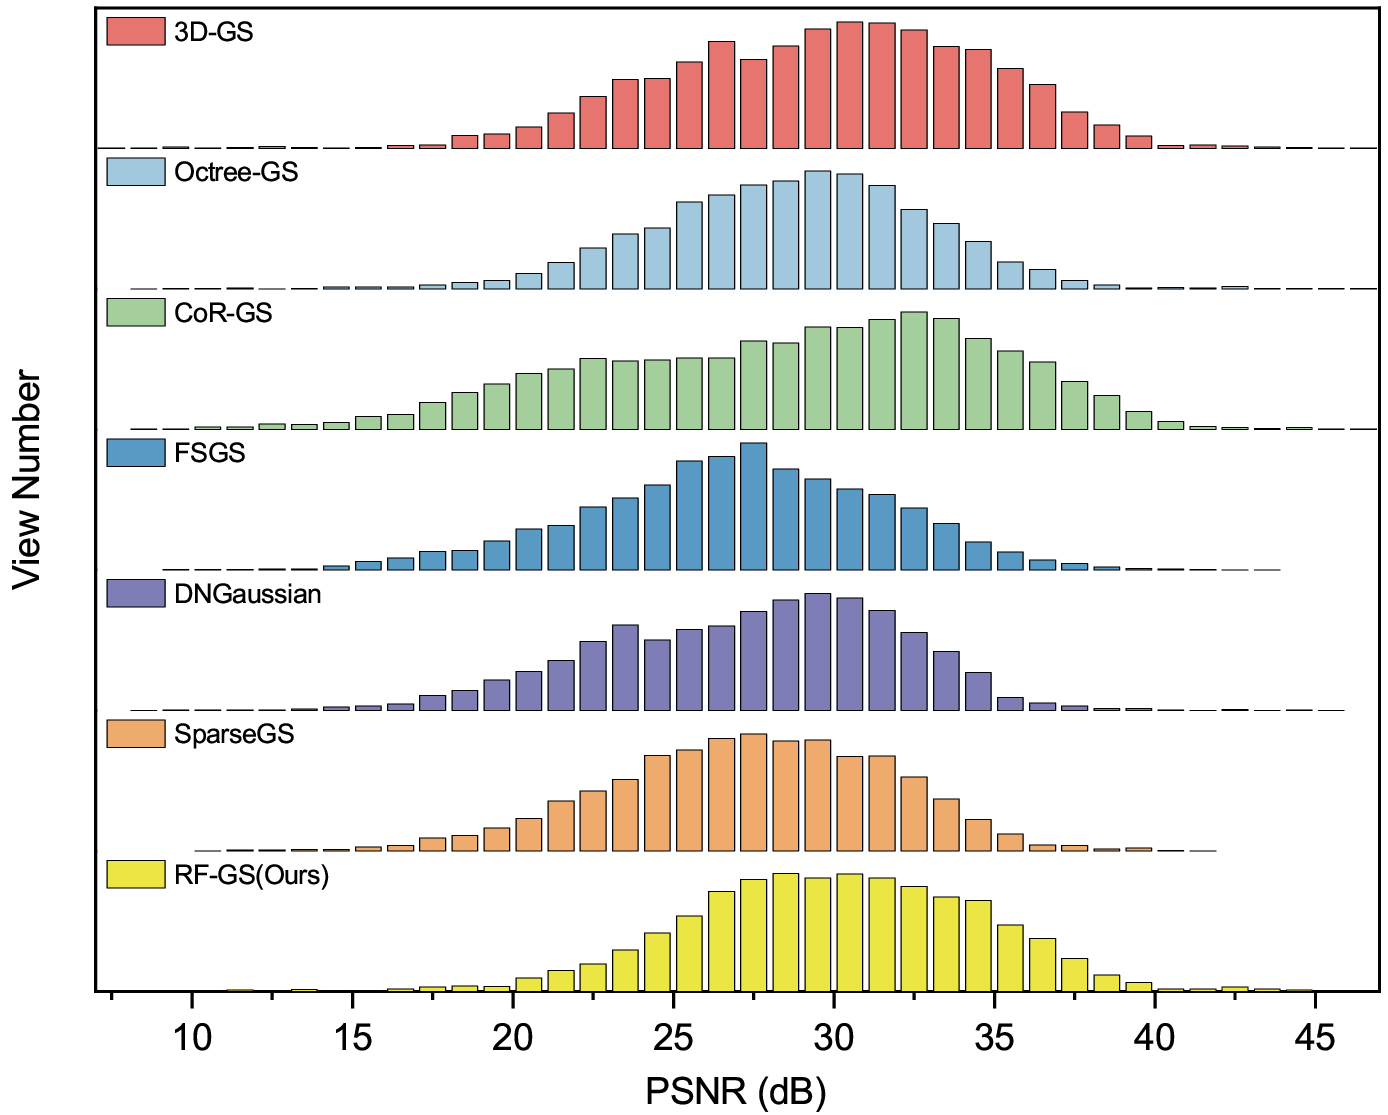}
	\end{minipage}
	\caption{Distribution of PSNR in simulated data. The figure shows the distribution of PSNR across 5449 test cases in a dense simulation scenario, with each algorithm marked by a distinct color. The x-axis represents PSNR values with a scale of 1, and the y-axis shows the number of test cases falling within each bin. Table 1 in the main text shows the standard deviation and mean.}
	\label{PSNR_DIS}
\end{figure}

\section{Explaination of Data Missing of SparseGS}

SparseGS is a neural rendering method based on a sparse voxel representation, which relies heavily on VRAM (graphics card memory) to store the voxel grid structure and optimize network parameters. While the method is designed to efficiently handle sparse voxel distributions, datasets like ScanNet++, with numerous overlapping viewpoints, necessitate higher voxel resolution to capture fine details. This results in a denser voxel grid and dramatically increases VRAM usage, exceeding 40 GiB in some cases. Additionally, SparseGS relies on well-covered camera trajectories to refine the sparse voxel distribution effectively. However, real-world data often feature simpler and less uniform trajectories, as shown in Figure \ref{data}, which can pose challenges for maintaining a balanced and memory-efficient voxel structure.

\begin{figure}[htp]
        \centering
	\begin{minipage}[c]{0.48\textwidth}
		\includegraphics[width=\textwidth]{sec/appendix/trajedy.pdf}
		\subcaption{}
		\label{data}
	\end{minipage}
    
	\begin{minipage}[c]{0.48\textwidth}
		\includegraphics[width=\textwidth, height=0.3\textwidth]{sec/appendix/sparseGS.pdf}
		\subcaption{}
		\label{sparseGS}
	\end{minipage} 

	\caption{Explaination of data missing of SparseGS. (a) represents the distribution of real captures generally distributed along the road. (b) represents the Gaussian representation obtained by sparseGS, geometrically degraded to an approximate plane.}
	\label{data missing}
\end{figure}

\section{The Impact of Training Data Density on NAFNet}
%为了探究当NAFNET基于点云投影图进行修复任务时，是否会因为训练数据的观测密度而造成图像恢复质量的大幅度变化，
To explore the relationship between the observation density of the training data and the quality of pseudo-view restoration when NAFNet performs the restoration task based on point projection images., as shown in Figure \ref{density}, we created a corridor scene and collected data at different densities along the same path to assess NAFNet's performance under different densities of observations. Since the actual pseudo-views are for weakly observed regions, we set up some wide-baseline test views, such as the blue squares in Fig. \ref{density}h, to ensure that the test results provide a valuable reference.

As shown in Figure \ref{density_result}, the quality of image restoration improves with increasing scene collection density, eventually converging to the model's performance upper limit. The rendering quality range indicates strong stability, with fluctuations within approximately 1 dB. This stability helps ensure a reliable lower bound for novel view synthesis quality under non-uniform observations.

\begin{figure}[htp]
        \centering
	\begin{minipage}[c]{0.49\textwidth}
		\includegraphics[width=\textwidth]{sec/appendix/diff_density_20241116202232.pdf}
	\end{minipage}

	\caption{Different sampling densities for viewpoints under the same path. (a)–(f) show sampling positions at different intervals, with camera frustums represented by red boxes. (g) illustrates the dimensions of the experimental scene, including the corridor's length, width, and height. (h) shows blue boxes representing wide-baseline views, used to evaluate the impact of different sampling densities on image reconstruction quality.}
	\label{density}
\end{figure}

\begin{figure}[htp]
        \centering
	\begin{minipage}[c]{0.23\textwidth}
		\includegraphics[width=\textwidth]{sec/appendix/train-view.pdf}
		\subcaption{}
		\label{density_result}
	\end{minipage}
	\begin{minipage}[c]{0.23\textwidth}
		\includegraphics[width=\textwidth]{sec/appendix/resolution.pdf}
		\subcaption{}
		\label{resolution}
	\end{minipage} 

	\caption{Stability evaluation of the image restoration model. (a) shows the impact of source view density on restoration quality, with each horizontal axis unit representing a station of four viewpoints, and the resolution of the point cloud is 5 mm. (b) shows the effect of point cloud resolution, with the horizontal axis indicating the distance between any two points.}
	\label{qulified result}
\end{figure}

\begin{figure}[htp]
        \centering
	\begin{minipage}[c]{0.15\textwidth}
		\includegraphics[width=\textwidth]{sec/appendix/gt.pdf}
		\subcaption{GT}
		\label{}
	\end{minipage}
	\begin{minipage}[c]{0.15\textwidth}
		\includegraphics[width=\textwidth]{sec/appendix/0.001.pdf}
		\subcaption{1 mm }
		\label{}
	\end{minipage} 
    	\begin{minipage}[c]{0.15\textwidth}
		\includegraphics[width=\textwidth]{sec/appendix/0.01.pdf}
		\subcaption{10 mm}
	\end{minipage} 

	\caption{Visulization of point projection in various resolutions of point clouds. As the resolution decreases, pixel spacing increases, leading to changes in the difference of image point projection.}
	\label{point_projection_img}
\end{figure}
\section{The Impact of Point Cloud Resolution on NAFNet}

%点投影图对点云的分辨率较为敏感，不同分辨率得到的投影图存在较大的视觉差异。因此我们进一步探究了NAFNet对点投影图进行恢复时，恢复质量与点云分辨率的关系。首先我们对\ref{density}a中的训练数据和\ref{density}h中的测试数据统一采用不同点云分辨率进行训练和修复，然后比较不同分辨率下的修复质量。
Point projection images are sensitive to the resolution of the point cloud, and there are large visual differences in the projection maps obtained from different resolutions, as shown in Figure \ref{point_projection_img}. Therefore, we explored the relationship between the recovery quality and point cloud resolution when NAFNet recovers point projection images. First, we train and restore the training data in \ref{density}a and the test data in \ref{density}h uniformly with different point cloud resolutions, then compare the restoration quality under various resolutions.

Figure \ref{resolution} shows that as the point cloud resolution decreases, there is no significant trend in PSNR, indicating that point cloud resolution has minimal impact on image restoration. This also demonstrates the robustness of the process from point projection to visible-light image.
